# Supplementary material for: Detection of the Orbital Hall Effect by the Orbital-Spin Conversion
Source: arXiv:2010.01970 source file (2020-10-05)
Supplement: Supplementary file 1 [file SM.pdf]

# Supplementary Materials for "Detection of the Orbital Hall Effect by the Orbital-Spin Conversion"

Jiewen Xiao,[1] Yizhou Liu,[1] and Binghai Yan[1,*]

[1] *Department of Condensed Matter Physics, Weizmann Institute of Science, Rehovot 7610001, Israel*

For the left lead 1 (yellow regime) shown in Figure S1, the Hamiltonian and orbital angular momentum operator can be written as

$$H_{lead}(k_x) = \begin{pmatrix} E_{onsite} & T & ... & ... & ... \\ T^\dagger & E_{onsite} & T & ... & ... \\ ... & T^\dagger & E_{onsite} & T & ... \\ ... & ... & T^\dagger & E_{onsite} & ... \\ ... & ... & ... & ... & ... \end{pmatrix} \tag{S1}$$

$$E_{onsite}(k_x) = \begin{pmatrix} E_s + 2t_s\cos(k_x a) & 0 & 0 \\ 0 & E_{px} + 2t_{p\sigma}\cos(k_x a) & 0 \\ 0 & 0 & E_{py} + 2t_{p\pi}\cos(k_x a) \end{pmatrix} \tag{S2}$$

$$T = \begin{pmatrix} t_s & 0 & t_{sp} \\ 0 & t_{p\pi} & 0 \\ -t_{sp} & 0 & t_{p\sigma} \end{pmatrix} \tag{S3}$$

$$L_{lead} = \begin{pmatrix} L_z & 0 & 0 & 0 & ... \\ 0 & L_z & 0 & 0 & ... \\ 0 & 0 & L_z & 0 & ... \\ 0 & 0 & 0 & L_z & ... \\ ... & ... & ... & ... & ... \end{pmatrix} \tag{S4}$$

In order to specify the orbital conductance in each $L_z$ channel, $L_{lead}$ is required to be a conserved a quantity, i.e., $L_{lead}$ commutes with the Hamiltonian. Therefore, the $[H_{lead}, L_{lead}] = 0$ commutation demands $[L_z, T] = 0$, which constrains $t_{sp} = 0$ eV, $t_{p\sigma} = t_{p\pi}$. For lead 2 and lead 3, the above restriction is still the same. Therefore, in the transport calculations, we set $t_{sp} = 0$ eV, $t_{p\sigma} = t_{p\pi} = 0.6$ eV in all leads. Other parameters are the same as the scattering region in the center. Furthermore, we shift the Fermi level in lead so that lead is a metal and $p_\pm$ orbitals will be infused and further polarized by the OHE. We also test the orbital non-conserved leads and results in Figure S4 display the similar feature as that in the main text.

---

* binghai.yan@weizmann.ac.il

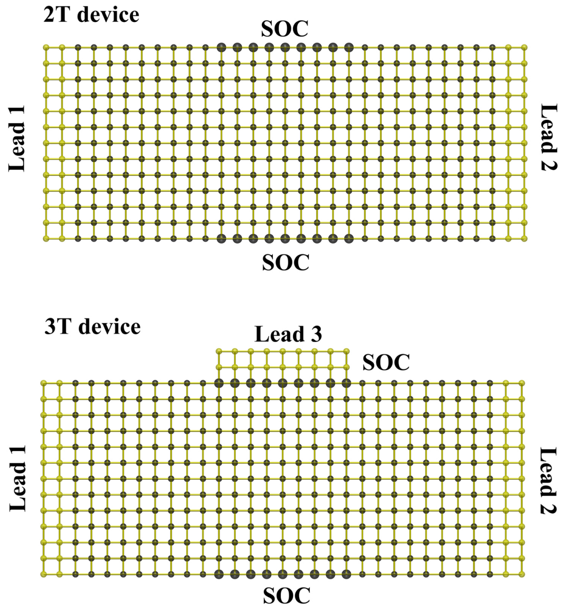


FIG. S1. 2T and 3T detection device based on the square lattice model.

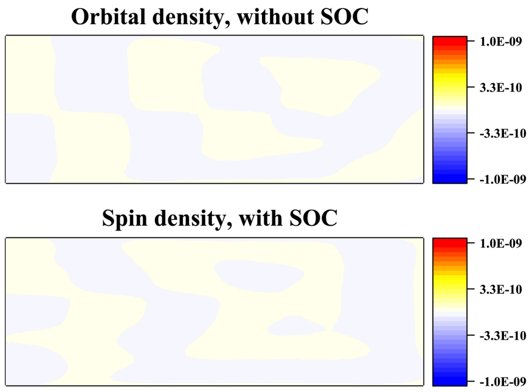


FIG. S2. Orbital density and spin density distribution in the 2T setup, at the energy level of 0.2 eV. $t_{sp}$ is set to 0.0 eV, which switches off the OHE. Therefore, it shows that SOC alone cannot generate the spin polarization.

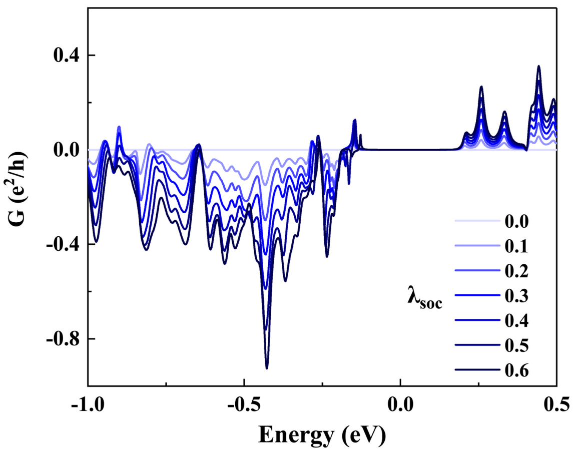


FIG. S3. Spin conductance in the 3T setup, with the increasing interfacial SOC strength.

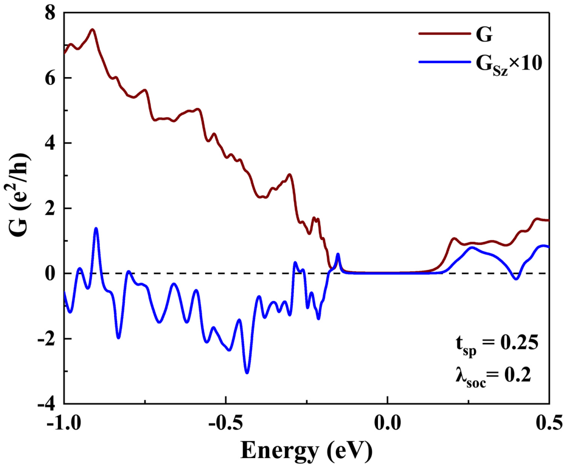


FIG. S4. Spin conductance for the orbital non-conserved leads, where $t_{sp}$ is set to 0.25 eV in all leads. Although $G_{Lz}$ cannot be defined, $G_{Sz}$ still displays the similar feature as that in Figure 2(d) in the main text.

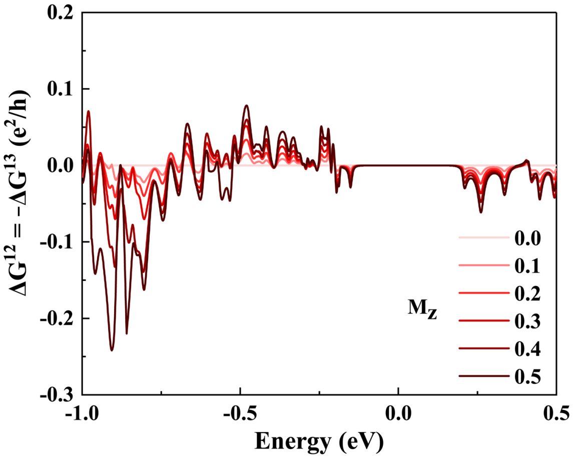


FIG. S5. $\Delta G^{12}$ and $\Delta G^{13}$ in the OHMR 3T setup, with the increasing exchange field $M_z$ in lead 3.

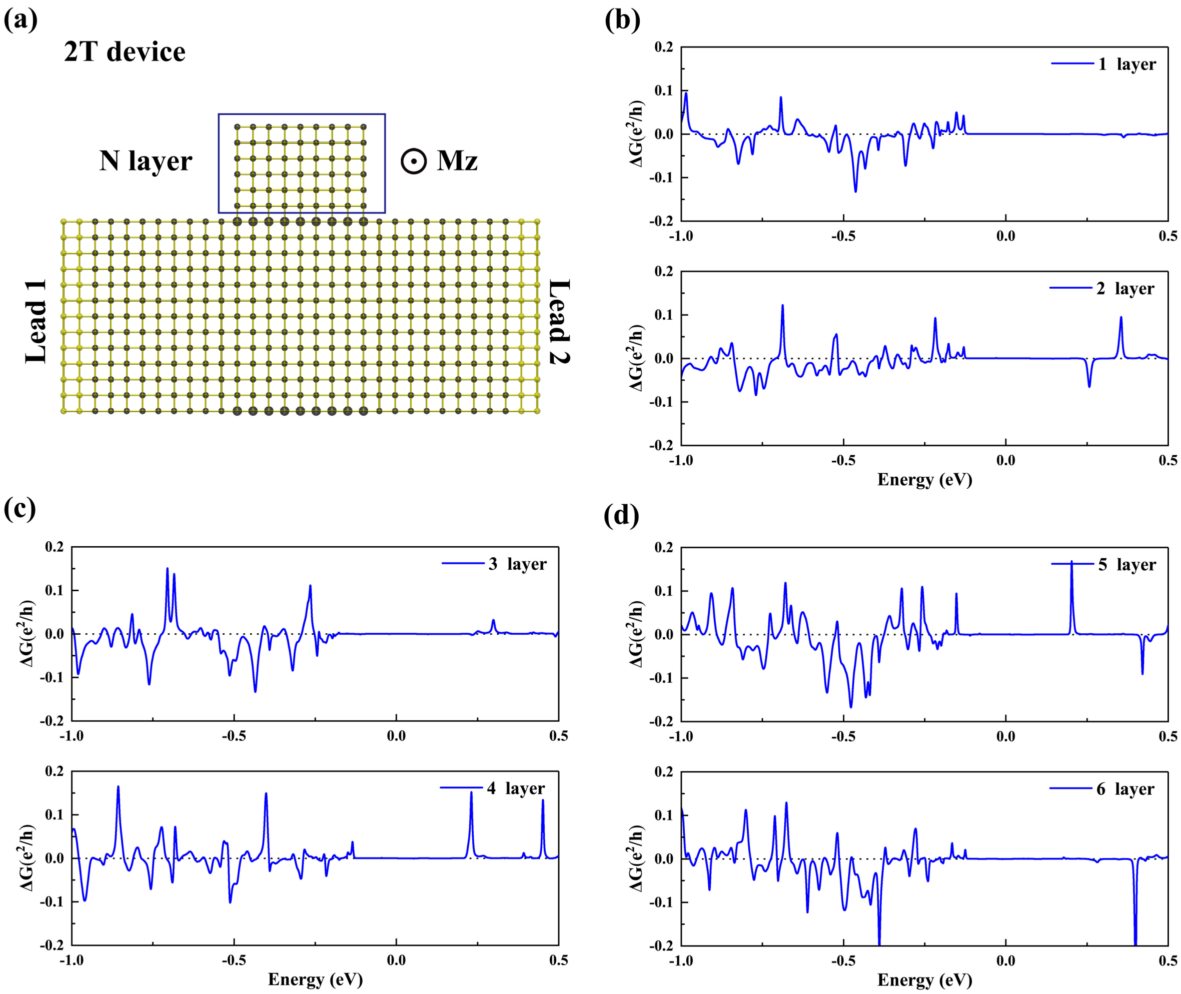


FIG. S6. (a) The 2T OHMR setup. As shown in the rectangular region, the size of the open lead is denoted as N layer, where exchange field is applied. The 2T OHMR ($\Delta G^{12}$) is calculated for N ranging from 1 to 6. (b) The 2T OHMR for 1 layer and 2 layer setup. (c) The 2T OHMR for 3 layer and 4 layer setup. (d) The 2T OHMR for 5 layer and 6 layer setup. In the main text, N is set to 3. In all these calculations, the dephasing term $\eta$ is set to 0.001. Therefore, from the above results, we can observe that the changing direction of $G_{12}$ in $\pm M_z$ field depends sensitively on the device geometry, due to the complex orbital accumulation and reflection in the open lead.

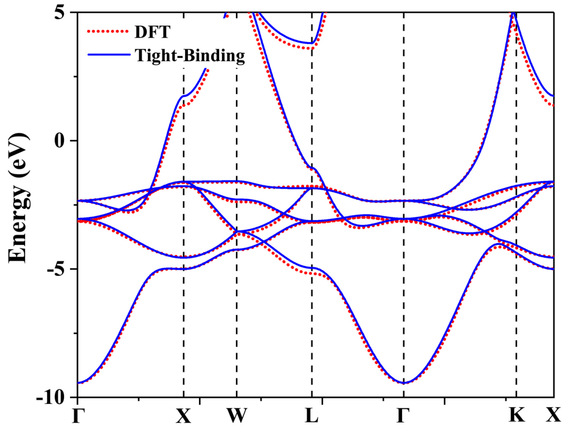


FIG. S7. Band structure of Cu based on DFT and tight-binding calculations.

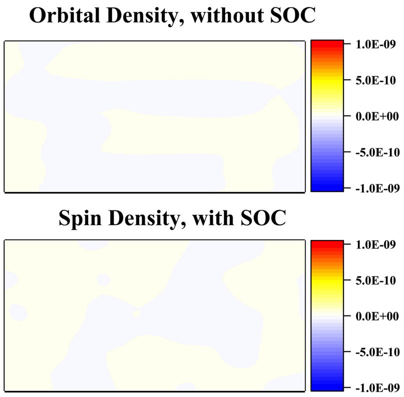


FIG. S8. Orbital and spin density distribution at the Fermi level in the 2T setup based on Cu. The inter-orbital hopping is artificially switched off. Results show that, without the OHE, the heavy metal Au with SOC alone cannot generate the spin polarization.

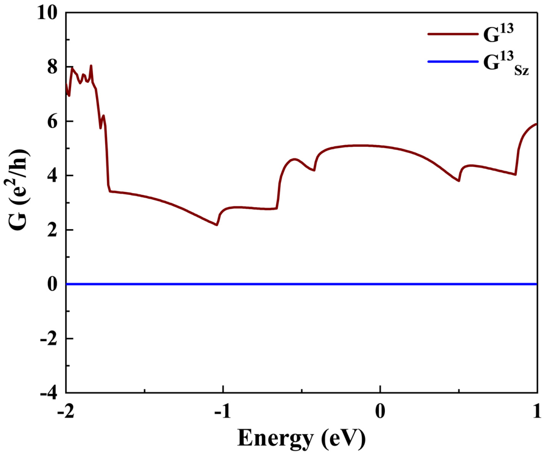


FIG. S9. Spin conductance $G^{13}_{S_z}$ in the 3T setup based on Cu, where the inter-orbital hopping is artificially switched off. Without the OHE, the heavy metal Au with SOC alone cannot generate the spin current.

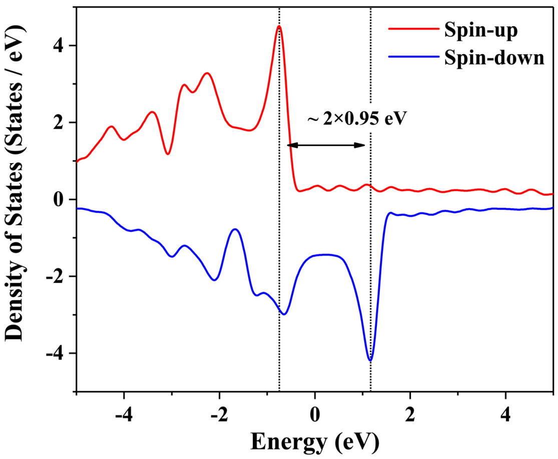


FIG. S10. Estimated exchange field in Co.
